# Supplementary material for: The ESO UVES Advanced Data Products Quasar Sample - VI. Sub-Damped Lyman-$\alpha$ Metallicity Measurements and the Circum-Galactic Medium
Source: arXiv:1602.02564 source file (2016-02-08)
Supplement: Supplementary file 1 [file QSOB0952-0115.tex]

Among the low ions, we detect no clear absorption profile. AlII 1670 present what seems to be a 5 components profile, but there is no other element to confirm that hypothesis so we did not performed any fit for the low ions. 

As for the high ions, we detect a $>3$ components profile in CIV 1548 and 1550, but no fit has been conducted due to a poor estimation of the continuum, CIV 1548 and 1550 being located on an emission line ($\lambda\sim1278$\AA in the quasar's restframe).
