# Supplementary material for: The ESO UVES Advanced Data Products Quasar Sample - VI. Sub-Damped Lyman-$\alpha$ Metallicity Measurements and the Circum-Galactic Medium
Source: arXiv:1602.02564 source file (2016-02-08)
Supplement: Supplementary file 4 [file tableSampleV3.tex]

\section[]{Sample}

This Appendix presents the full list of damped absorbers identified in the EUADP, including estimates of their metallicity from various references.

XXX mettre a jour la table avec les nouvelles metallicite solaire


\onecolumn




%\centering
%\caption{Part of the EUADPQ sample that has been studied in metallicity}
\begin{longtable}{lcccccc}
\hline
\hline
QSO name & $z_{\rm em}$& $z_{\rm abs}$ & log NHI & [X/H] & X & Reference for metallicity measurements\\ 
\hline
\endfirsthead
\multicolumn{7}{c}%
{\tablename\ \thetable\ -- \textit{Continued from previous page}} \\
\hline\hline
QSO name & $z_{\rm em}$ & $z_{\rm abs}$ & log NHI & [X/H] & X &  Reference for metallicity measurements \\ 
\hline
\endhead
\hline \multicolumn{7}{r}{\textit{Continued on next page}} \\
\endfoot
\hline
\endlastfoot

QSO J0003-2323 & 2.1870 & $19.60\pm0.40$ & $-1.76\pm0.42$ & OI & \cite{Richter2005} \ 
Q0005+0524 & 0.8514 & $19.08\pm0.04$ & $-0.43\pm0.18$ & FeII & \cite{Meiring2009} \ 
QSO J0006-6208 & 2.9700 & $20.70\pm0.00$ & $0.00\pm0.00$ & no & \cite{Peroux2005} \ 
QSO J0006-6208 & 3.2020 & $20.80\pm0.10$ & $0.00\pm0.00$ & no & \cite{Peroux2005} \ 
QSO J0006-6208 & 3.7760 & $21.00\pm0.00$ & $0.00\pm0.00$ & no & \cite{Peroux2005} \ 
QSO J0006-6208 & 4.1450 & $19.37\pm0.15$ & $0.00\pm0.00$ & no & \cite{Peroux2005} \ 
QSO J0008-2900 & 2.2540 & $20.22\pm0.10$ & $-1.58\pm0.21$ & FeII & This work \ 
QSO J0008-2901 & 2.4910 & $19.94\pm0.11$ & $-1.38\pm0.21$ & SII & This work \ 
QSO J0008-0958 & 1.7680 & $20.85\pm0.15$ & $-0.31\pm0.17$ & ZnII & Herbert-Fort06 \ 
LBQS 0009-0138 & 1.3860 & $20.26\pm0.02$ & $-1.32\pm0.04$ & SiII & \cite{Meiring2009} \ 
LBQS 0010-0012 & 2.0250 & $20.95\pm0.10$ & $-1.26\pm0.12$ & ZnII & Ledoux03,Srianand05 \ 
Q0012-0122 & 1.3862 & $20.26\pm0.02$ & $-1.34\pm0.08$ & SiII & \cite{Meiring2009} \ 
LBQS 0013-0029 & 1.9730 & $20.83\pm0.05$ & $-0.65\pm0.06$ & ZnII & Petitjean02 \ 
LBQS 0018+0026 & 0.5200 & $19.54\pm0.03$ & $-1.51\pm0.19$ & FeII & Ellison08 \ 
LBQS 0018+0026 & 0.9400 & $19.38\pm0.15$ & $0.10\pm0.24$ & FeII & Ellison08 \ 
J001855-091351 & 0.5840 & $20.11\pm0.10$ & $-1.38\pm0.21$ & FeII & This work \ 
Q0021+0104 & 1.3259 & $20.04\pm0.11$ & $-0.49\pm0.21$ & FeII & \cite{Meiring2009} \ 
Q0021+0104 & 1.5756 & $20.48\pm0.15$ & $-1.11\pm0.15$ & SiII & \cite{Meiring2009} \ 
J0021+0043 & 0.9424 & $19.38\pm0.13$ & $0.54\pm0.26$ & FeII & Dessauges09 \ 
QSO B0027-1836 & 2.4020 & $21.75\pm0.10$ & $-1.52\pm0.10$ & ZnII & Noterdaeme07 \ 
QSO B0039-3354 & 2.2240 & $20.60\pm0.10$ & $-1.27\pm0.11$ & SiII & Noterdaeme08 \ 
J004054.7-091526 & 4.7400 & $20.55\pm0.15$ & $-1.93\pm0.15$ & SiII & Becker11,Rafelski12 \ 
J0040-0915 & 4.7394 & $20.30\pm0.15$ & $-1.39\pm0.24$ & FeII & \cite{Rafelski2012} \ 
QSO J0041-4936 & 2.2480 & $20.46\pm0.13$ & $-1.32\pm0.16$ & ZnII & This work \ 
LBQS 0042-2930 & 1.8090 & $20.40\pm0.10$ & $-1.21\pm0.12$ & SiII & \cite{Fox2009} \ 
LBQS 0042-2930 & 1.9360 & $20.50\pm0.10$ & $-1.23\pm0.11$ & SiII & \cite{Fox2009} \ 
QSO B0058-292 & 2.6710 & $21.10\pm0.10$ & $-1.43\pm0.11$ & ZnII & Ledoux03,Srianand05 \ 
QSO B0100+1300 & 2.3090 & $21.35\pm0.08$ & $-1.42\pm0.08$ & ZnII & Prochaska98,Dessauges03 \ 
QSO J0105-1846 & 2.3700 & $21.00\pm0.08$ & $-1.79\pm0.14$ & ZnII & Ledoux03,Srianand05 \ 
QSO J0105-1846 & 2.9260 & $20.00\pm0.10$ & $-1.56\pm0.13$ & OI & Noterdaeme08 \ 
QSO B0112-30 & 2.4180 & $20.50\pm0.08$ & $-2.24\pm0.11$ & OI & Petitjean08 \ 
QSO B0112-30 & 2.7020 & $20.30\pm0.10$ & $-0.44\pm0.13$ & SiII & Ledoux03,Srianand05 \ 
QSO B0122-005 & 1.7610 & $20.78\pm0.07$ & $-0.87\pm0.11$ & SiII & Ellison09 \ 
QSO B0122-005 & 2.0100 & $20.04\pm0.07$ & $-1.88\pm0.09$ & SiII & Ellison09 \ 
QSO J0123-0058 & 1.4090 & $20.08\pm0.09$ & $-0.41\pm0.13$ & ZnII & \cite{Peroux2008} \ 
QSO J0124+0044 & 2.9880 & $19.18\pm0.10$ & $-0.57\pm0.16$ & SiII & Peroux07 \ 
QSO J0124+0044 & 3.0780 & $20.21\pm0.10$ & $-0.59\pm0.40$ & SiII & Peroux07 \ 
QSO B0128-2150 & 1.8570 & $20.21\pm0.09$ & $-1.00\pm0.09$ & SII & This work \ 
J013209-082349 & 0.6470 & $20.60\pm0.12$ & $-0.78\pm0.23$ & FeII & This work \ 
QSO J0133+0400 & 3.1390 & $19.01\pm0.10$ & $0.00\pm0.00$ & no & Peroux07 \ 
QSO J0133+0400 & 3.6920 & $20.68\pm0.15$ & $-0.96\pm0.16$ & SiII & Prochaska03 \ 
QSO J0133+0400 & 3.7730 & $20.55\pm0.13$ & $-0.59\pm0.13$ & SiII & Prochaska03 \ 
QSO J0133+0400 & 3.9950 & $19.94\pm0.15$ & $-1.54\pm0.20$ & SiII & Peroux07 \ 
QSO J0133+0400 & 3.9990 & $19.16\pm0.15$ & $0.00\pm0.00$ & no & Peroux07 \ 
QSO J0133+0400 & 4.0210 & $19.09\pm0.15$ & $0.00\pm0.00$ & no & Peroux07 \ 
QSO J0134+0051 & 0.8420 & $19.93\pm0.13$ & $-0.60\pm0.22$ & FeII & Peroux06 \ 
QSO B0135-42 & 3.1010 & $19.81\pm0.10$ & $-1.21\pm0.27$ & SiII & Peroux07 \ 
QSO B0135-42 & 3.6650 & $19.11\pm0.10$ & $-2.42\pm0.16$ & OI & Peroux07 \ 
QSO J0138-0005 & 0.7820 & $19.81\pm0.09$ & $0.32\pm0.10$ & ZnII & \cite{Peroux2008} \ 
QSO J0153+0009 & 0.7710 & $19.70\pm0.09$ & $0.00\pm0.00$ & no & \cite{Peroux2008} \ 
QSO J0157-0048 & 1.4160 & $19.90\pm0.07$ & $-0.34\pm0.10$ & ZnII & Ellison08 \ 
QSO B0201+113 & 3.3850 & $21.26\pm0.08$ & $-1.17\pm0.14$ & SII & Ellison01 \ 
QSO J0209+0517 & 3.6660 & $20.47\pm0.10$ & $-1.97\pm0.21$ & FeII & Prochaska03 \ 
QSO J0209+0517 & 3.7070 & $19.24\pm0.10$ & $0.00\pm0.00$ & no & \cite{Peroux2005} \ 
QSO J0209+0517 & 3.8630 & $20.55\pm0.10$ & $-2.60\pm0.11$ & SiII & Prochaska03 \ 
QSO B0216+0803 & 1.7690 & $20.20\pm0.10$ & $-0.86\pm0.12$ & ZnII & Lu96 \ 
QSO B0216+0803 & 2.2930 & $20.45\pm0.16$ & $-0.54\pm0.17$ & ZnII & Lu96,Vladilo11 \ 
QSO J0217+0144 & 1.3450 & $19.89\pm0.09$ & $-1.11\pm0.10$ & MgII & Bergeron86,Blades82 \ 
QSO B0237-2322 & 1.3650 & $19.30\pm0.30$ & $0.08\pm0.30$ & SiII & Srianand07 \ 
QSO B0237-2322 & 1.6720 & $19.65\pm0.10$ & $-0.37\pm0.13$ & ZnII & Ellison12 \ 
QSO B0244-1249 & 1.8630 & $19.48\pm0.18$ & $-0.79\pm0.27$ & SiII & Ellison09 \ 
QSO B0253+0058 & 0.7250 & $20.70\pm0.17$ & $-0.07\pm0.17$ & ZnII & Peroux06 \ 
QSO B0254-404 & 2.0460 & $20.45\pm0.08$ & $-1.43\pm0.09$ & SII & Noterdaeme08 \ 
QSO B0307-195B & 1.7880 & $19.00\pm0.10$ & $0.49\pm0.10$ & SiII & This work \ 
QSO J0332-4455 & 2.6560 & $19.82\pm0.05$ & $-1.67\pm0.06$ & OI & Fox07 \ 
QSO B0335-122 & 3.1780 & $20.80\pm0.07$ & $-2.77\pm0.10$ & SiII & Akerman05,Noterdaeme08 \ 
QSO B0336-017 & 3.0620 & $21.20\pm0.09$ & $-1.33\pm0.09$ & SII & Prochaska01 \ 
0338-0005 & 2.9090 & $21.10\pm0.10$ & $-1.03\pm0.10$ & SII & Prochaska07 \ 
QSO B0347-383 & 3.0250 & $20.63\pm0.09$ & $-0.96\pm0.15$ & ZnII & Prochaska01,Ledoux03 \ 
QSO B0347-2111 & 1.9470 & $20.30\pm0.10$ & $0.00\pm0.00$ & no & Akerman05 \ 
QSO J0354-2724 & 1.4050 & $20.18\pm0.15$ & $-0.01\pm0.15$ & ZnII & \cite{Meiring2007} \ 
QSO J0407-4410 & 1.9130 & $20.80\pm0.10$ & $-0.92\pm0.11$ & ZnII & Ledoux06 \ 
QSO J0407-4410 & 2.5510 & $21.13\pm0.10$ & $-1.25\pm0.11$ & ZnII & Lopez03,Srianand05 \ 
QSO J0407-4410 & 2.5950 & $21.09\pm0.10$ & $-0.97\pm0.10$ & ZnII & Lopez03,Srianand05 \ 
QSO J0407-4410 & 2.6210 & $20.45\pm0.10$ & $-1.95\pm0.10$ & OI & Lopez03,Srianand05 \ 
QSO J0422-3844 & 3.0820 & $19.37\pm0.02$ & $-0.69\pm0.04$ & OI & Carswell96 \ 
QSO J0427-1302 & 1.5620 & $19.35\pm0.10$ & $-2.26\pm0.21$ & FeII & This work \ 
QSO J0427-1302 & 1.4080 & $19.04\pm0.04$ & $-0.99\pm0.06$ & SiII & \cite{Meiring2009} \ 
QSO B0432-440 & 2.2970 & $20.78\pm0.10$ & $0.00\pm0.00$ & no & Akerman05 \ 
QSO B0438-43 & 2.3470 & $20.78\pm0.12$ & $-0.62\pm0.12$ & ZnII & Akerman05 \ 
PKS 0439-433 & 0.1012 & $19.63\pm0.15$ & $0.28\pm0.15$ & SII & Kulkarni14 \ 
QSO B0449-1645 & 1.0070 & $20.98\pm0.07$ & $-0.92\pm0.10$ & ZnII & \cite{Peroux2008} \ 
QSO B0450-1310B & 2.0670 & $20.50\pm0.07$ & $-2.13\pm0.08$ & OI & Dessauges05,Zafar13 \ 
PKS 0454-220 & 0.4740 & $19.45\pm0.03$ & $0.47\pm0.04$ & SII & This work, Kulkarni14, Rao06, Som15 \ 
4C-02.19 & 2.0400 & $21.70\pm0.10$ & $-1.13\pm0.10$ & ZnII & Heinmuller06 \ 
QSO B0512-3329 & 0.9310 & $20.49\pm0.08$ & $-1.16\pm0.21$ & FeII & Lopez05 \ 
QSO B0515-4414 & 1.1510 & $19.88\pm0.05$ & $-0.22\pm0.06$ & ZnII & Quast08,Zych08 \ 
QSO B0528-2505 & 2.1410 & $20.70\pm0.08$ & $-0.26\pm0.09$ & ZnII & Lu96,Centurion03 \ 
QSO B0528-2505 & 2.8110 & $21.35\pm0.07$ & $-0.82\pm0.10$ & ZnII & Srianand98,Lu96 \ 
QSO B0551-36 & 1.9620 & $20.70\pm0.08$ & $-0.24\pm0.09$ & ZnII & Ledoux02 \ 
J060008.1-504036 & 2.1490 & $20.40\pm0.12$ & $-0.85\pm0.12$ & ZnII & This work \ 
QSO B0642-5038 & 2.6590 & $20.95\pm0.08$ & $-1.01\pm0.10$ & ZnII & Noterdaeme08,Zafar13 \ 
J0747+4434 & 4.0196 & $20.95\pm0.15$ & $-2.40\pm0.25$ & NiII & \cite{Rafelski2012} \ 
J0759+1800 & 4.6577 & $20.85\pm0.15$ & $-1.71\pm0.16$ & SII & \cite{Rafelski2012} \ 
J0817+1351 & 4.2584 & $21.30\pm0.15$ & $-1.12\pm0.15$ & SII & \cite{Rafelski2012} \ 
J0825+3544 & 3.2073 & $20.30\pm0.10$ & $-1.67\pm0.21$ & FeII & \cite{Rafelski2012} \ 
J0825+3544 & 3.6567 & $21.25\pm0.10$ & $-1.83\pm0.13$ & SiII & \cite{Rafelski2012} \ 
J0825+5127 & 3.3180 & $20.85\pm0.10$ & $-1.67\pm0.14$ & SiII & \cite{Rafelski2012} \ 
Q0826-2230 & 0.9110 & $19.04\pm0.04$ & $1.11\pm0.09$ & ZnII & \cite{Meiring2009} \ 
QSO B0827+2421 & 0.5180 & $20.30\pm0.04$ & $-0.85\pm0.19$ & FeII & \cite{Meiring2006} \ 
J0831+4046 & 4.3440 & $20.75\pm0.15$ & $-2.36\pm0.15$ & SiII & \cite{Rafelski2012} \ 
J0834+2140 & 3.7102 & $20.85\pm0.10$ & $-1.55\pm0.21$ & FeII & \cite{Rafelski2012} \ 
J0834+2140 & 4.3900 & $21.00\pm0.20$ & $-1.27\pm0.20$ & SII & \cite{Rafelski2012} \ 
J0834+2140 & 4.4610 & $20.30\pm0.15$ & $-1.86\pm0.16$ & SiII & \cite{Rafelski2012} \ 
J0839+3524 & 4.2800 & $20.30\pm0.15$ & $-1.14\pm0.24$ & FeII & \cite{Rafelski2012} \ 
QSO B0841+129 & 1.8640 & $21.00\pm0.10$ & $-1.30\pm0.11$ & SII & Ledoux06 \ 
QSO B0841+129 & 2.3750 & $21.05\pm0.10$ & $-1.50\pm0.11$ & ZnII & Prochaska98,Zafar13 \ 
QSO B0841+129 & 2.4760 & $20.80\pm0.10$ & $-1.67\pm0.11$ & ZnII & Prochaska98,Dessauges05 \ 
J0909+3303 & 3.6584 & $20.55\pm0.10$ & $-1.16\pm0.11$ & SII & \cite{Rafelski2012} \ 
QSO B0913+0715 & 2.6180 & $20.35\pm0.10$ & $-2.41\pm0.10$ & OI & Pettini08,Petitjean08 \ 
J0925+4004 & 0.2477 & $19.55\pm0.15$ & $-0.29\pm0.17$ & OI & \cite{Battisti2012} \ 
J0928+6025 & 0.1538 & $19.35\pm0.15$ & $0.41\pm0.25$ & FeII & \cite{Battisti2012} \ 
QSO B0933-333 & 2.6820 & $20.50\pm0.10$ & $-1.22\pm0.12$ & SiII & Akerman05,Noterdaeme08 \ 
QSO B0951-0450 & 3.2350 & $20.25\pm0.10$ & $-1.97\pm0.10$ & SiII & Prochaska03 \ 
QSO B0951-0450 & 3.8580 & $20.60\pm0.10$ & $-1.47\pm0.10$ & SiII & Prochaska98 \ 
QSO B0951-0450 & 4.2030 & $20.55\pm0.10$ & $-2.63\pm0.34$ & OI & Prochaska98 \ 
QSO B0952+179 & 0.2380 & $21.32\pm0.05$ & $-0.95\pm0.06$ & ZnII & Kulkarni05 \ 
QSO B0952-0115 & 4.0240 & $20.55\pm0.10$ & $-2.61\pm0.11$ & SiII & Prochaska01 \ 
J1001+5944 & 0.3035 & $19.32\pm0.10$ & $-0.37\pm0.10$ & OI & \cite{Battisti2012} \ 
QSO J1009-0026 & 0.8400 & $20.20\pm0.07$ & $-0.97\pm0.19$ & FeII & \cite{Meiring2007} \ 
QSO J1009-0026 & 0.8800 & $19.48\pm0.08$ & $0.34\pm0.09$ & ZnII & \cite{Meiring2007} \ 
J1009+0713 & 0.1140 & $20.68\pm0.10$ & $-0.55\pm0.16$ & SII & \cite{Battisti2012} \ 
J1013+4240 & 4.7979 & $20.60\pm0.15$ & $-2.14\pm0.15$ & SiII & \cite{Rafelski2012} \ 
J1017+6116 & 2.7684 & $20.60\pm0.10$ & $-2.71\pm0.10$ & OI & \cite{Rafelski2012} \ 
LBQS 1026-0045B & 0.6320 & $19.95\pm0.07$ & $-0.05\pm0.17$ & ZnII & Ellison08 \ 
LBQS 1026-0045B & 0.7090 & $20.04\pm0.06$ & $-0.08\pm0.19$ & FeII & Ellison08 \ 
J1028-0100 & 0.6321 & $19.95\pm0.07$ & $-0.01\pm0.21$ & FeII & Dessauges09 \ 
J1028-0100 & 0.7089 & $20.04\pm0.06$ & $-0.06\pm0.20$ & FeII & Dessauges09 \ 
QSO B1036-2257 & 2.5330 & $19.30\pm0.10$ & $-1.33\pm0.10$ & MgII & This work \ 
QSO B1036-2257 & 2.7770 & $20.93\pm0.05$ & $-1.26\pm0.05$ & SII & Prochaska03 \ 
Q1037+0028 & 1.4244 & $20.04\pm0.12$ & $-0.46\pm0.12$ & SiII & \cite{Meiring2009} \ 
QSO J1039-2719 & 2.1390 & $19.70\pm0.05$ & $-0.17\pm0.06$ & ZnII & Srianand01 \ 
J1042+3107 & 4.0865 & $20.75\pm0.10$ & $-1.95\pm0.10$ & SiII & \cite{Rafelski2012} \ 
QSO B1045+056 & 0.9510 & $19.28\pm0.02$ & $-0.93\pm0.20$ & FeII & \cite{Meiring2006} \ 
J1051+3107 & 4.1392 & $20.70\pm0.20$ & $-1.96\pm0.22$ & SII & \cite{Rafelski2012} \ 
J1051+3545 & 4.3498 & $20.45\pm0.10$ & $-1.88\pm0.10$ & SiII & \cite{Rafelski2012} \ 
J1051+3545 & 4.8206 & $20.35\pm0.10$ & $-2.28\pm0.10$ & SiII & \cite{Rafelski2012} \ 
Q1054-0020 & 0.8301 & $18.95\pm0.18$ & $0.24\pm0.25$ & FeII & \cite{Meiring2009} \ 
Q1054-0020 & 0.9514 & $19.28\pm0.02$ & $-0.76\pm0.18$ & FeII & \cite{Meiring2009} \ 
QSO B1055-301 & 1.9040 & $21.54\pm0.10$ & $-1.19\pm0.10$ & ZnII & Akerman05 \ 
J1100+1122 & 4.3947 & $21.74\pm0.10$ & $-1.67\pm0.22$ & FeII & \cite{Rafelski2012} \ 
QSO B1101-26 & 1.8380 & $19.50\pm0.05$ & $-1.64\pm0.10$ & OI & \cite{Dessauges-Zavadsky2003} \ 
J1101+0531 & 4.3446 & $21.30\pm0.10$ & $-1.07\pm0.12$ & SiII & \cite{Rafelski2012} \ 
QSO B1104-181 & 1.6610 & $20.85\pm0.01$ & $-0.93\pm0.01$ & ZnII & Lopez99 \ 
QSO J1107+0048 & 0.7400 & $21.00\pm0.04$ & $-0.50\pm0.16$ & ZnII & Peroux06,Zych08 \ 
Q1107+0003 & 0.9542 & $20.26\pm0.14$ & $0.00\pm0.00$ & no & \cite{Nestor2008} \ 
QSO B1108-07 & 3.4820 & $19.95\pm0.07$ & $-1.57\pm0.09$ & SiII & Ledoux06 \ 
QSO B1108-07 & 3.6080 & $20.37\pm0.07$ & $-1.69\pm0.08$ & OI & Prochaska01,Petitjean08 \ 
J1111+3509 & 4.0520 & $20.80\pm0.15$ & $-1.95\pm0.16$ & SiII & \cite{Rafelski2012} \ 
QSO J1113-1533 & 3.2650 & $21.30\pm0.05$ & $-1.61\pm0.07$ & ZnII & Ledoux06,Zafar13 \ 
QSO B1122-168 & 0.6820 & $20.45\pm0.05$ & $-3.23\pm0.06$ & MgII & Ledoux02b \ 
QSO B1151+068 & 1.7750 & $21.30\pm0.08$ & $-1.52\pm0.11$ & ZnII & \cite{Pettini1997b} \ 
J115538.6+053050 & 3.3270 & $21.00\pm0.10$ & $-0.81\pm0.10$ & SII & This work \ 
J1155+3510 & 2.7582 & $21.00\pm0.10$ & $-1.35\pm0.10$ & SII & \cite{Rafelski2012} \ 
J1200+4015 & 3.2200 & $20.85\pm0.10$ & $-0.55\pm0.11$ & ZnII & \cite{Rafelski2012} \ 
J1200+4618 & 4.4765 & $20.50\pm0.15$ & $-1.37\pm0.24$ & FeII & \cite{Rafelski2012} \ 
J1201+2117 & 3.7975 & $21.35\pm0.15$ & $-0.75\pm0.15$ & SiII & \cite{Rafelski2012} \ 
J1201+2117 & 4.1578 & $20.60\pm0.15$ & $-2.38\pm0.15$ & SiII & \cite{Rafelski2012} \ 
QSO B1202-074 & 4.3830 & $20.49\pm0.16$ & $-1.59\pm0.17$ & SiII & Lu96a \ 
J1202+3235 & 4.7955 & $21.10\pm0.15$ & $-2.34\pm0.24$ & FeII & \cite{Rafelski2012} \ 
J1202+3235 & 5.0647 & $20.30\pm0.15$ & $-2.66\pm0.16$ & SiII & \cite{Rafelski2012} \ 
J120550.2+020131 & 1.7470 & $20.40\pm0.10$ & $-0.88\pm0.13$ & ZnII & \cite{Fox2009} \ 
QSO B1209+0919 & 2.5840 & $21.40\pm0.10$ & $-0.98\pm0.11$ & ZnII & Prochaska07 \ 
LBQS 1210+1731 & 1.8920 & $20.70\pm0.08$ & $-0.89\pm0.09$ & ZnII & Prochaska01,Dessauges05 \ 
Q1215-0034 & 1.5543 & $19.56\pm0.02$ & $-0.31\pm0.18$ & FeII & \cite{Meiring2009} \ 
PG1216+069 & 0.0063 & $19.32\pm0.03$ & $-1.69\pm0.06$ & OI & Tripp05 \ 
QSO B1220-1800 & 2.1120 & $20.12\pm0.07$ & $-0.71\pm0.08$ & SII & Noterdaeme08 \ 
Q1220-0040 & 0.9746 & $20.20\pm0.07$ & $-1.00\pm0.19$ & FeII & \cite{Meiring2009} \ 
LBQS 1223+1753 & 2.4660 & $21.40\pm0.10$ & $-1.41\pm0.10$ & ZnII & Prochaska01,Srianand05 \ 
LBQS 1223+1753 & 2.5570 & $19.32\pm0.15$ & $-0.45\pm0.15$ & SiII & \cite{Dessauges-Zavadsky2003} \ 
PHL 1226 & 0.1602 & $19.48\pm0.10$ & $0.24\pm0.15$ & SII & Kulkarni14 \ 
QSO B1228-113 & 2.1930 & $20.60\pm0.10$ & $-0.15\pm0.11$ & ZnII & Akerman05 \ 
Q1228+1018 & 0.9376 & $19.41\pm0.02$ & $0.03\pm0.18$ & FeII & \cite{Meiring2009} \ 
QSO B1230-101 & 1.9310 & $20.48\pm0.10$ & $-0.10\pm0.11$ & ZnII & Akerman05 \ 
LBQS 1232+0815 & 1.7200 & $19.48\pm0.13$ & $-0.58\pm0.13$ & SiII & This work \ 
LBQS 1232+0815 & 2.3340 & $20.70\pm0.04$ & $-0.62\pm0.10$ & ZnII & Srianand00,Ge01,Zafar13 \ 
J1238+3437 & 2.4714 & $20.80\pm0.10$ & $-2.01\pm0.15$ & SII & \cite{Rafelski2012} \ 
J1241+4617 & 2.6674 & $20.70\pm0.10$ & $-2.18\pm0.10$ & SiII & \cite{Rafelski2012} \ 
LBQS 1246-0217 & 1.7810 & $21.45\pm0.00$ & $-1.00\pm0.05$ & ZnII & Herbert-Fort06 \ 
J1248+3110 & 3.6973 & $20.60\pm0.10$ & $-1.63\pm0.21$ & FeII & \cite{Rafelski2012} \ 
J1253+1046 & 4.6001 & $20.30\pm0.15$ & $-1.35\pm0.24$ & FeII & \cite{Rafelski2012} \ 
J1257-0111 & 4.0208 & $20.30\pm0.10$ & $-1.56\pm0.10$ & SiII & \cite{Rafelski2012} \ 
J1304+1202 & 2.9131 & $20.55\pm0.15$ & $-1.62\pm0.16$ & SII & \cite{Rafelski2012} \ 
J1304+1202 & 2.9289 & $20.30\pm0.15$ & $-1.51\pm0.16$ & SII & \cite{Rafelski2012} \ 
J1323-0021 & 0.7160 & $20.21\pm0.20$ & $0.66\pm0.21$ & ZnII & Peroux06a \ 
QSO J1330-2522 & 2.6540 & $19.56\pm0.13$ & $-1.73\pm0.21$ & AlII & This work \ 
Q1330-2056 & 0.8526 & $19.40\pm0.02$ & $-0.74\pm0.18$ & FeII & \cite{Meiring2009} \ 
QSO B1331+170 & 1.7760 & $21.15\pm0.07$ & $-1.10\pm0.07$ & ZnII & Prochaska98,Dessauges03 \ 
QSO J1342-1355 & 3.1180 & $20.05\pm0.08$ & $-1.22\pm0.08$ & OI & Pretitjean08 \ 
J1353+5328 & 2.8349 & $20.80\pm0.10$ & $-1.35\pm0.10$ & SII & \cite{Rafelski2012} \ 
QSO J1356-1101 & 2.3970 & $19.85\pm0.08$ & $-1.55\pm0.20$ & FeII & This work \ 
QSO J1356-1101 & 2.5010 & $20.44\pm0.05$ & $-1.29\pm0.10$ & SII & Akerman05,Noterdaeme08 \ 
QSO J1356-1101 & 2.9670 & $20.80\pm0.10$ & $-1.35\pm0.12$ & SiII & Akerman05,Noterdaeme08 \ 
QSO B1409+0930 & 2.0190 & $20.65\pm0.10$ & $-1.58\pm0.14$ & ZnII & Ledoux08 \ 
QSO B1409+0930 & 2.4560 & $20.53\pm0.08$ & $-2.07\pm0.10$ & OI & Pettini02 \ 
QSO B1409+0930 & 2.6680 & $19.80\pm0.08$ & $-1.18\pm0.14$ & OI & Pettini02,dessauges03 \ 
J1412+0624 & 4.1095 & $20.40\pm0.15$ & $-1.71\pm0.25$ & FeII & \cite{Rafelski2012} \ 
QSO J1421-0643 & 3.4480 & $20.40\pm0.10$ & $-1.29\pm0.13$ & SiII & Akerman05,Noterdaeme08 \ 
J1435+3604 & 0.2026 & $19.80\pm0.10$ & $-0.32\pm0.16$ & SII & \cite{Battisti2012} \ 
Q1436-0051 & 0.7377 & $20.08\pm0.11$ & $0.03\pm0.12$ & ZnII & \cite{Meiring2009} \ 
J1438+4314 & 4.3990 & $20.89\pm0.15$ & $-1.28\pm0.15$ & SII & \cite{Rafelski2012} \ 
QSO J1439+1117 & 2.4180 & $20.10\pm0.10$ & $0.27\pm0.11$ & ZnII & Noterdaeme08 \ 
QSO J1443+2724 & 4.2240 & $20.95\pm0.10$ & $-0.52\pm0.10$ & ZnII & Prochaska01,Noterdaeme08,Ledoux06 \ 
LBQS 1444+0126 & 2.0870 & $20.25\pm0.07$ & $-0.69\pm0.17$ & ZnII & Ledoux03,dessauges03 \ 
Q1455-0045 & 1.0929 & $20.08\pm0.06$ & $-0.95\pm0.12$ & SiII & \cite{Meiring2009} \ 
J1507+4406 & 3.0644 & $20.75\pm0.10$ & $-1.90\pm0.14$ & SII & \cite{Rafelski2012} \ 
J1541+3153 & 2.4435 & $20.95\pm0.10$ & $-1.48\pm0.15$ & ZnII & \cite{Rafelski2012} \ 
J1553+3548 & 0.0830 & $19.55\pm0.15$ & $-0.84\pm0.16$ & SiII & \cite{Battisti2012} \ 
PHL 1598 & 0.4297 & $19.18\pm0.03$ & $0.01\pm0.09$ & SII & Kulkarni14 \ 
J1607+1604 & 4.4741 & $20.30\pm0.15$ & $-1.71\pm0.15$ & SiII & \cite{Rafelski2012} \ 
J1616+4154 & 0.3211 & $20.60\pm0.20$ & $-0.35\pm0.23$ & SII & \cite{Battisti2012} \ 
J1619+3342 & 0.0963 & $20.55\pm0.10$ & $-0.59\pm0.13$ & SII & \cite{Battisti2012} \ 
QSO J1621-0042 & 3.1040 & $19.70\pm0.20$ & $-1.43\pm0.20$ & SiII & This work \ 
J1626+2751 & 4.3110 & $21.34\pm0.15$ & $-1.15\pm0.24$ & FeII & \cite{Rafelski2012} \ 
J1626+2751 & 4.4975 & $21.39\pm0.15$ & $-2.45\pm0.24$ & FeII & \cite{Rafelski2012} \ 
J1626+2751 & 5.1791 & $20.94\pm0.15$ & $-1.46\pm0.15$ & SII & \cite{Rafelski2012} \ 
4C 12.59 & 0.5310 & $20.70\pm0.09$ & $-1.58\pm0.22$ & FeII & This work \ 
4C 12.59 & 0.9000 & $19.70\pm0.04$ & $-0.67\pm0.19$ & FeII & \cite{Meiring2009} \ 
J1654+2227 & 4.0022 & $20.60\pm0.15$ & $-1.65\pm0.24$ & FeII & \cite{Rafelski2012} \ 
QSO J1723+2243 & 3.6970 & $20.35\pm0.10$ & $0.00\pm0.00$ & no & Prochaska03 \ 
QSO B2000-330 & 3.1720 & $19.75\pm0.15$ & $-2.29\pm0.15$ & OI & Prochter10 \ 
QSO B2000-330 & 3.1880 & $19.80\pm0.15$ & $-1.34\pm0.15$ & SiII & Prochter10 \ 
QSO B2000-330 & 3.1920 & $19.10\pm0.15$ & $-0.48\pm0.15$ & SiII & Prochter10 \ 
Q2051+1950 & 1.1157 & $20.00\pm0.15$ & $0.34\pm0.18$ & ZnII & \cite{Meiring2009} \ 
LBQS 2114-4347 & 1.9120 & $19.50\pm0.10$ & $-0.70\pm0.10$ & MgII & This work \ 
QSO J2119-3536 & 1.9960 & $20.10\pm0.07$ & $-0.36\pm0.11$ & ZnII & \cite{Dessauges-Zavadsky2003} \ 
QSO B2126-15 & 2.6380 & $19.25\pm0.15$ & $-0.09\pm0.15$ & SiII & This work \ 
QSO B2126-15 & 2.7690 & $19.20\pm0.15$ & $0.08\pm0.15$ & SiII & This work \ 
LBQS 2132-4321 & 1.9160 & $20.74\pm0.09$ & $-0.61\pm0.09$ & ZnII & This work \ 
LBQS 2138-4427 & 2.3830 & $20.60\pm0.05$ & $-1.11\pm0.09$ & ZnII & Ledoux06 \ 
LBQS 2138-4427 & 2.8520 & $20.98\pm0.05$ & $-1.55\pm0.07$ & ZnII & Ledoux03,Srianand05 \ 
Q2149+212 & 1.0023 & $19.30\pm0.05$ & $0.00\pm0.00$ & no & \cite{Nestor2008} \ 
LBQS 2206-1958A & 1.9210 & $20.67\pm0.05$ & $-0.32\pm0.05$ & ZnII & Prochaska01,Vladilo11 \ 
LBQS 2206-1958A & 2.0760 & $20.44\pm0.05$ & $-2.08\pm0.06$ & OI & Pettini08 \ 
QSO B2222-396 & 2.1540 & $20.85\pm0.10$ & $-1.72\pm0.12$ & SII & Noterdaeme08 \ 
LBQS 2230+0232 & 1.8640 & $20.90\pm0.10$ & $-0.66\pm0.10$ & ZnII & Prochaska98,Dessauges05 \ 
QSO B2237-0607 & 4.0790 & $20.55\pm0.10$ & $-1.79\pm0.10$ & SiII & Lu96 \ 
J223941.8-294955 & 1.8250 & $18.84\pm0.14$ & $1.36\pm0.15$ & ZnII & Zafar14_prep \ 
J2252+1425 & 4.7475 & $20.60\pm0.15$ & $-1.76\pm0.26$ & FeII & \cite{Rafelski2012} \ 
QSO B2311-373 & 2.1820 & $20.48\pm0.13$ & $-1.45\pm0.15$ & SiII & Akerman05,Noterdaeme08 \ 
QSO B2318-1107 & 1.6290 & $20.52\pm0.14$ & $-1.52\pm0.23$ & FeII & This work \ 
QSO B2318-1107 & 1.9890 & $20.68\pm0.05$ & $-0.74\pm0.06$ & ZnII & Noterdaeme07 \ 
QSO J2328+0022 & 0.6520 & $20.32\pm0.07$ & $-0.45\pm0.17$ & ZnII & Peroux06 \ 
QSO B2332-094 & 3.0570 & $20.50\pm0.07$ & $-1.24\pm0.07$ & OI & Ledoux03,Prochaska03,Petitjean08,Zafar13 \ 
J233544.2+150118 & 0.6800 & $19.70\pm0.30$ & $0.11\pm0.30$ & ZnII & \cite{Peroux2008} \ 
QSO B2343+125 & 2.4310 & $20.40\pm0.07$ & $-0.76\pm0.10$ & ZnII & Noterdaeme07 \ 
QSO J2346+1247 & 2.5690 & $20.98\pm0.04$ & $-0.66\pm0.07$ & ZnII & Rix07 \ 
QSO B2348-0180 & 2.4260 & $20.50\pm0.10$ & $-0.56\pm0.14$ & SII & Noterdaeme07a,Dessaugses05 \ 
QSO B2348-0180 & 2.6150 & $21.30\pm0.08$ & $-1.92\pm0.11$ & SiII & Prochaska01 \ 
QSO B2348-147 & 2.2790 & $20.56\pm0.08$ & $-1.95\pm0.14$ & SII & Prochaska98,Dessauges07 \ 
Q2352-0028 & 0.8730 & $19.18\pm0.09$ & $-0.84\pm0.20$ & FeII & \cite{Meiring2009} \ 
Q2352-0028 & 1.0318 & $19.81\pm0.13$ & $0.17\pm0.13$ & SiII & \cite{Meiring2009} \ 
Q2352-0028 & 1.2467 & $19.60\pm0.24$ & $-0.53\pm0.30$ & FeII & \cite{Meiring2009} \ 
LBQS 2359-0216 & 2.0950 & $20.65\pm0.10$ & $-0.61\pm0.10$ & ZnII & Prochaska98 \ 
LBQS 2359-0216 & 2.1540 & $20.30\pm0.10$ & $-1.49\pm0.10$ & SiII & Prochaska98 \ 





\end{longtable}

\twocolumn
